# Supplementary material for: Superconducting quantum node for entanglement and storage of microwave radiation
Source: arXiv:1401.5622 ancillary file (2015-02-04)
Supplement: Supplementary file 1 [file Flurin-PRL-SupInfo.pdf]

# Supplementary material: Superconducting quantum node for entanglement and storage of microwave radiation

E. Flurin, N. Roch, J.D. Pillet, F. Mallet, and B. Huard\*

*Laboratoire Pierre Aigrain, Ecole Normale Supérieure-PSL Research University,*

*CNRS, Université Pierre et Marie Curie-Sorbonne Universités,*

*Université Paris Diderot-Sorbonne Paris Cité, 24 rue Lhomond, 75231 Paris Cedex 05, France*

(Dated: February 4, 2015)

PACS numbers:

## MEASUREMENT SETUP

Pump and drive pulses are generated by modulation of continuous microwave tones produced by microwave generators set respectively at  $f_a - f_m + 70$  MHz for the conversion pump,  $f_a + f_m + 100$  MHz for the entangling pump and  $f_a + 40$  MHz for the input drive (see Fig. S1). The amplitude modulation shaping is performed by mixing these tones with arbitrary shaped waveforms at 70, 100 and 40 MHz synthesized by a 4 channels Tektronix Arbitrary Waveform Generator (AWG5014B). The FPGA board is an X6-RX by Innovative integration with 16-bit deep ADCs at 160 MSps. All clocks and triggers are carefully synchronized together.

Pump pulses and drive pulse are sent into the dilution refrigerator through separated input lines which are thermalized, attenuated and filtered with cryogenic components at each stage ensuring that only negligible thermal excitations enter the device. The pump lines are then recombined with a diplexer and sent to the sum port of the 180 degree hybrid coupler which distribute the field on the common mode of the Josephson Ring Modulator. The drive line is sent to the differential port of the hybrid through the  $-20$  dB port of a directional coupler.

The output signal is collected on the differential port of the 180-hybrid coupler is routed back towards a commercial High Electron Mobility Transistor (HEMT) amplifier of 40 dB gain from Caltech University through two isolators in series. The output signal is further amplified and filtered at room temperature, mixed down by the microwave source at  $f_a + 40$  MHz, filtered and amplified on a 125MHz bandwidth FEMTO amplifier. The output signal is then digitalized, demodulated and averaged in real time by the FPGA board on a 550 ns time window.

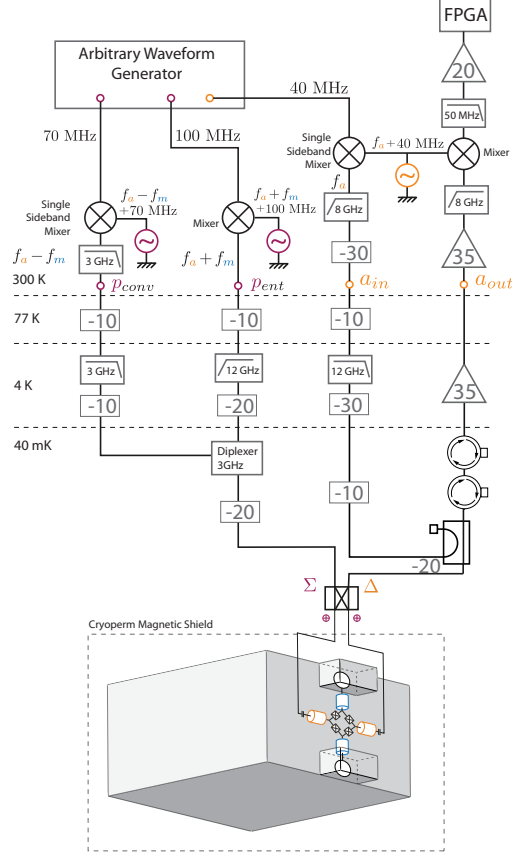

Figure S1: Detailed measurement setup. The gray rectangles stand for microwave attenuators. The gray triangles are HEMT amplifiers.

## TUNABILITY AND PARTICIPATION RATIO

### Tunability

The buffer and cavity modes can be modeled as  $LC$  resonators inductively coupled to the Josephson Ring Modulator (JRM) (see Fig. S3). The Josephson ring modulator consists in a ring of four identical Josephson junctions threaded by a magnetic flux  $\Phi_{ext} = \varphi_{ext}\varphi_0$ . Then  $L_{JRM}(\varphi_{ext}) = \frac{L_J^0}{\cos \varphi/4}$  with  $L_J^0$  is the zero-flux inductance of the Josephson junctions. The equivalent inductance of modes  $a$  and  $m$  is made of the JRM inductance  $L_{JRM}(\varphi_{ext})$  in series with the geometric inductance  $L_{a,m}$ . Consequently by varying the magnetic flux threading the JRM, we tune the frequency of the resonator  $f_{a,m} = (2\pi\sqrt{(L_{a,m} + L_{JRM}(\varphi_{ext}))C_{a,m}})^{-1}$ .

The experimental tunability of the buffer resonator is presented on the figure S2. The frequency is tunable over 800 MHz in the range  $f_a = 8.8 \text{ GHz} - 9.6 \text{ GHz}$ . This tunability is stronger than in similar devices used for amplification [1, 2] due to a lower critical current  $I_c = 1.1 \mu\text{A}$  of the junctions. Here, we want to maximize the participation ratio even if it degrades the dynamical range. Note that in the context of a quantum memory, large dynamical ranges are more easily achieved since the resonators don't have to sustain high photon power as a consequence of the high amplification gain.

Note that around  $\varphi_{ext} \approx 0.8\pi$ , we observe an anti-crossing in the resonance frequency of about 10 MHz. It is certainly due to the coupling to a two level system (TLS) trapped in the oxide of one of the junction. The frequency of the TLS is moving from one cool down to another.

On the other hand, the 3D cavity frequency is tunable over 200 kHz only. Indeed, the participation ratio of the JRM in the total equivalent inductance of the 3D cavity is much smaller, the scaling factor being  $0.2/800 = 2.5 \times 10^{-4}$ .

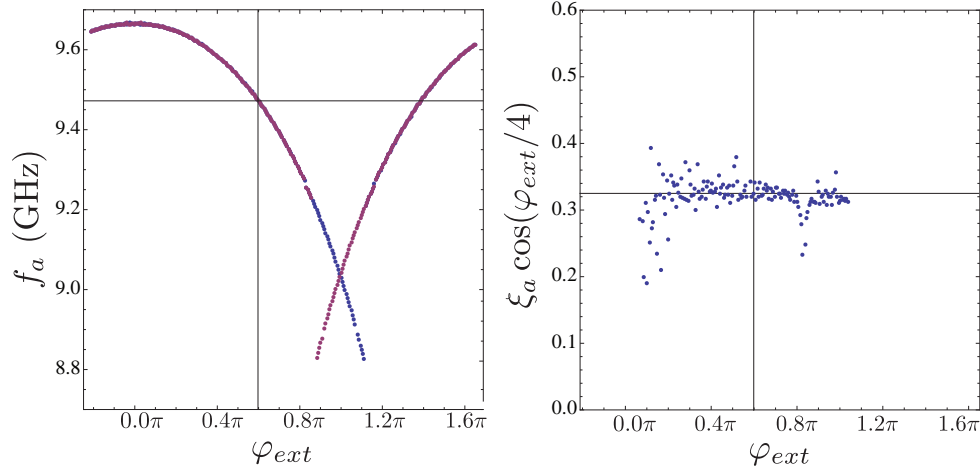

Figure S2: Left panel: resonance frequency of the buffer mode  $f_a$  as a function of reduced flux through the ring  $\varphi_{ext}$ . The blue dots are measured with increasing field while the purple dots are measured with decreasing field. Right panel: Scaled participation ratio of JRM in the buffer cavity  $\xi_a \cos(\varphi_{ext}/4)$  as a function of  $\varphi_{ext}$  inferred from Eq. (S3) using the measurement in the left panel.

### Stability

We can show that for flux bias  $\varphi_{ext} > \pi$ , the JRM becomes metastable and can jump to another flux configuration by accepting an extra flux quantum into the ring. This metastability presents a hysteric behavior, ramping the flux up and down the jump from one configuration to another happen at a different flux bias as presented figure S2. Note that for a good stability of the device, it is preferable to work at flux point away from half flux quantum  $\varphi_{ext} = \pi$ . In the present experiment we are working at  $\varphi_{ext} \approx 0.6\pi$ .

### Participation ratios

We define the participation ratio  $\xi_{a,m}$  as the ratio of the zero-flux inductance of the Josephson Ring Modulator (JRM) to the total inductance of the mode  $a$  (or  $m$ ). For mode  $a$ ,

$$\xi = \frac{L_{JRM}(\varphi_{ext})}{L_{tot}(\varphi_{ext})} \quad (S1)$$

where  $L_{tot} = L_a + L_{JRM}(\varphi_{ext})$ . We can show that relative variation of the resonance frequency  $f_a$  is directly link to the participation ratio.

$$\left| \frac{1}{f_a} \frac{\partial f_a}{\partial \varphi_{ext}} \right| = \left| \frac{1}{2L_{tot}} \frac{\partial L_{tot}}{\partial \varphi_{ext}} \right| = \frac{\xi_0 \tan(\varphi_{ext}/4)}{8 \cos(\varphi_{ext}/4)} \quad (S2)$$

where  $\xi_0 = L_{JRM}(0)/L_{tot}(\varphi_{ext})$  is almost flux independent and is given by

$$\xi_0 = 2 \frac{\cos(\varphi/4)}{\tan(\varphi/4)} \left| \frac{1}{f} \frac{\partial f}{\partial \varphi} \right|. \quad (S3)$$

On Fig. S2, it can be seen that the right hand side of this equation is indeed almost independent on flux. Finally, we get the following expression for the participation ratio

$$\xi(\varphi_{ext}) = \frac{2}{\tan(\varphi_{ext}/4)} \left| \frac{1}{f} \frac{\partial f}{\partial \varphi_{ext}} \right|. \quad (S4)$$

As shown on figure S2, using this relation we just derived, we get a participation ratio for the buffer resonator of  $\xi_a \approx 0.35$ . We can estimate the participation ratio of the 3D cavity mode knowing the scaling factor between the frequency ranges over which the buffer and the memory modes are tunable. We get  $\xi_m \approx (0.2/800) 0.3 \approx 10^{-4}$ .

## CONSTRAINTS ON DEVICE PARAMETERS

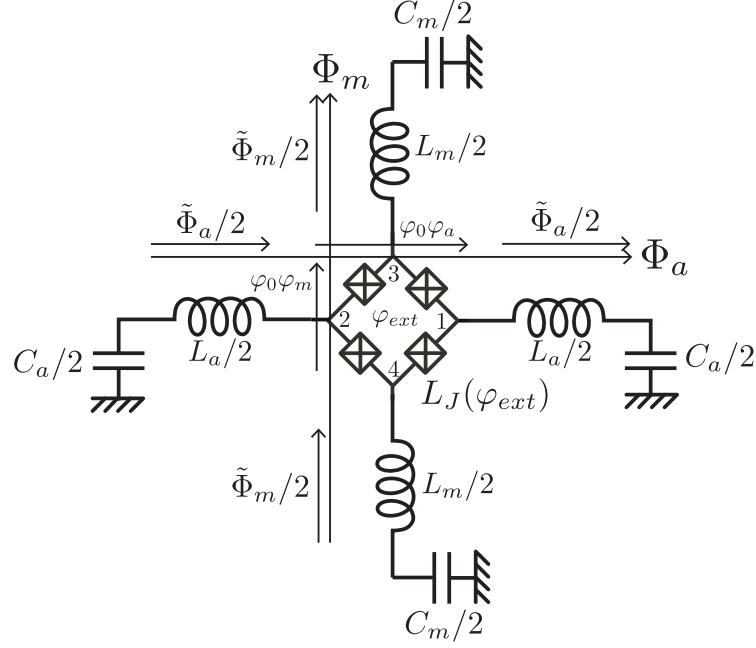

Figure S3: Schematics of the equivalent circuit used in the model.

From the Kirchhoff laws, we can deduce the following relation between fluxes for both resonators  $a$  and  $m$ .

$$\begin{cases} \Phi_a = \tilde{\Phi}_a + \varphi_0\varphi_a \\ \frac{\tilde{\Phi}_a}{L_a} = \frac{\varphi_0\varphi_a}{L_{JRM}} = \frac{\varphi_0\varphi_a}{L_J(\varphi_{ext})} \end{cases} \quad (\text{S5})$$

$$\begin{cases} \Phi_m = \tilde{\Phi}_m + \varphi_0\varphi_m \\ \frac{\tilde{\Phi}_m}{L_m} = \frac{\varphi_0\varphi_m}{L_{JRM}} = \frac{\varphi_0\varphi_m}{L_J(\varphi_{ext})} \end{cases} \quad (\text{S6})$$

Thus,

$$\begin{cases} \varphi_0\varphi_a = \frac{L_{JRM}}{L_a + L_{JRM}}\Phi_a \equiv \xi_a(\varphi_{ext})\Phi_a \\ \varphi_0\varphi_m = \frac{L_{JRM}}{L_m + L_{JRM}}\Phi_m \equiv \xi_m(\varphi_{ext})\Phi_m \end{cases} \quad (\text{S7})$$

$$\begin{cases} \tilde{\Phi}_a = \frac{L_a}{L_a + L_{JRM}}\Phi_a = (1 - \xi_a(\varphi_{ext}))\Phi_a \\ \tilde{\Phi}_m = \frac{L_m}{L_m + L_{JRM}}\Phi_m = (1 - \xi_m(\varphi_{ext}))\Phi_m \end{cases} \quad (\text{S8})$$

The Josephson Hamiltonian for a single junction reads  $H_J = -\frac{\varphi_0^2}{L_J} \cos \varphi$  where  $\varphi$  is the phase difference operator. The full Hamiltonian of the JRM can then be rewritten as a function of the reduced fluxes  $\varphi_a = \varphi_1 - \varphi_2$ ,  $\varphi_m = \varphi_3 - \varphi_4$  and  $\varphi_p = \varphi_1 + \varphi_2 - \varphi_3 - \varphi_4$  where  $\varphi_{1,2,3,4}$  are the flux of each node of the JRM [3]:

$$H = \frac{Q_a^2}{2C_a} + \frac{\tilde{\Phi}_a^2}{2L_a} + \frac{Q_m^2}{2C_m} + \frac{\tilde{\Phi}_m^2}{2L_m} - 4\frac{\varphi_0^2}{L_J^0} \left( \cos \frac{\varphi_{ext}}{4} \cos \frac{\varphi_a}{2} \cos \frac{\varphi_m}{2} \cos \frac{\varphi_p}{2} + \sin \frac{\varphi_{ext}}{4} \sin \frac{\varphi_a}{2} \sin \frac{\varphi_m}{2} \sin \frac{\varphi_p}{2} \right). \quad (S9)$$

We then expand this Hamiltonian at the third order in  $\varphi$

$$H = \frac{Q_a^2}{2C_a} + \frac{\tilde{\Phi}_a^2}{2L_a} + \frac{Q_m^2}{2C_m} + \frac{\tilde{\Phi}_m^2}{2L_m} + \frac{\varphi_0^2}{2L_J^0} \cos \frac{\varphi_{ext}}{4} (\varphi_a^2 + \varphi_m^2 + \varphi_p^2) - \frac{\varphi_0^2}{2L_J^0} \sin \frac{\varphi_{ext}}{4} \varphi_a \varphi_m \varphi_p + O(\varphi^3). \quad (S10)$$

Using Eqs. (S7) and (S8), we can then express the full Hamiltonian as a function of the total fluxes  $\Phi_a$  and  $\Phi_m$  and as a function of the participation ratio  $\xi_a$  and  $\xi_m$ .

$$\begin{aligned} H &= \frac{Q_a^2}{2C_a} + \frac{\tilde{\Phi}_a^2}{2L_a} + \frac{Q_m^2}{2C_m} + \frac{\tilde{\Phi}_m^2}{2L_m} + \frac{\varphi_0^2}{2L_J(\varphi_{ext})} (\varphi_a^2 + \varphi_m^2 + \varphi_p^2) - \frac{\varphi_0^2}{2L_J^0} \sin \frac{\varphi_{ext}}{4} \varphi_a \varphi_m \varphi_p \\ &= \frac{Q_a^2}{2C_a} + \frac{\Phi_a^2}{2(L_a + L_J(\varphi_{ext}))} + \frac{Q_m^2}{2C_m} + \frac{\Phi_m^2}{2(L_m + L_J(\varphi_{ext}))} - \frac{1}{2L_J^0} \frac{L_J(\varphi_{ext})}{L_a + L_J(\varphi_{ext})} \frac{L_J(\varphi_{ext})}{L_m + L_J(\varphi_{ext})} \sin \frac{\varphi_{ext}}{4} \Phi_a \Phi_m \varphi_p \\ &= \frac{Q_a^2}{2C_a} + \frac{\Phi_a^2}{2(L_a + L_J(\varphi_{ext}))} + \frac{Q_m^2}{2C_m} + \frac{\Phi_m^2}{2(L_m + L_J(\varphi_{ext}))} - \frac{1}{2L_J^0} \xi_a(\varphi_{ext}) \xi_m(\varphi_{ext}) \sin \frac{\varphi_{ext}}{4} \Phi_a \Phi_m \varphi_p. \end{aligned}$$

Finally, we can rewrite this Hamiltonian using the ladder operators  $\varphi_a = \sqrt{\hbar Z_a/2}(a + a^\dagger)$  and  $\varphi_m = \sqrt{\hbar Z_m/2}(m + m^\dagger)$  and  $\varphi_p = \varphi_{ZPF}^p(p + p^*)$ . Here  $Z_{a,m} = \sqrt{L_{a,m} + L_J(\varphi_{ext})}/\sqrt{C_{a,m}}$  and  $\omega_{a,m} = 1/\sqrt{L_{a,m}C_{a,m} + L_J(\varphi_{ext})C_{a,m}}$ .

$$H = \hbar\omega_a(a^\dagger a + \frac{1}{2}) + \hbar\omega_m(m^\dagger m + \frac{1}{2}) \quad (S11)$$

$$- \frac{\hbar}{2} \frac{\varphi_{ZPF}^p}{2L_J^0} \xi_a(\varphi_{ext}) \xi_m(\varphi_{ext}) \sqrt{Z_a Z_m} (a + a^\dagger)(m + m^\dagger)(p + p^*) \sin \frac{\varphi_{ext}}{4}. \quad (S12)$$

By identifying this Hamiltonian with the three-wave mixing Hamiltonian, we get the coupling term  $\chi$  as function of physical quantities of the circuit.

$$H = \hbar\omega_a(a^\dagger a + \frac{1}{2}) + \hbar\omega_m(m^\dagger m + \frac{1}{2}) - \hbar\chi(a + a^\dagger)(m + m^\dagger)(p + p^*), \quad (S13)$$

with

$$\chi = \frac{\varphi_{ZPF}^p}{4L_J^0} \xi_a \xi_m \sin \frac{\varphi_{ext}}{4} \sqrt{Z_a Z_m} \quad (S14)$$

$$= \frac{\varphi_{ZPF}^p}{4L_J^0} \xi_a \xi_m \sin \frac{\varphi_{ext}}{4} \sqrt{(L_a + L_J)(L_m + L_J)} \omega_a \omega_m \quad (S15)$$

$$\boxed{\chi = \frac{\varphi_{ZPF}^p}{4} \tan \frac{\varphi_{ext}}{4} \sqrt{\xi_a \xi_m \omega_a \omega_m}} \quad (S16)$$

The third order expansion of the Hamiltonian holds as long as the pump power is not too large. The constraint on the pump amplitude is then:

$$\varphi_{ZPF}^p |p| = \varphi_p \ll 2\pi. \quad (S17)$$

However, in order to reach the strong coupling regime, where the input/output rate  $\gamma_{io}$  reaches its maximum value, we need:

$$1 < \frac{2\chi|p|}{\kappa_a} \quad (S18)$$

By combining these two relations, we get the following constraint on the participation ratio the frequencies and the coupling rate to the transmission line:

$$1 \ll \frac{4\pi\chi}{\varphi_{ZPF}^p \kappa_a} = \pi \tan \frac{\varphi_{ext}}{4} \frac{\sqrt{\xi_a \xi_m \omega_a \omega_m}}{\kappa_a} \quad (\text{S19})$$

$$\boxed{1 \ll 2\pi^2 \tan \frac{\varphi_{ext}}{4} \frac{\sqrt{\xi_a \xi_m f_a f_m}}{\kappa_a}} \quad (\text{S20})$$

The constraint is satisfied in the physical implementation of the device.

$$2\pi^2 \tan \frac{\varphi_{ext}}{4} \frac{\sqrt{\xi_a \xi_m f_a f_m}}{\kappa_a} = 2\pi^2 \tan\left(\frac{\pi}{2}0.3\right) \frac{\sqrt{0.3 \times 10^{-4} \times 9.4 \times 7.8}}{2\pi \times 0.007 \times \cos(\frac{\pi}{2}0.3)} \approx 12 \gg 1 \quad (\text{S21})$$

## KERR EFFECT

The pump amplitude is varied in time to turn the memory on and off. It was therefore important to know by how much the pump power affects the resonance frequency of the buffer and memory modes. This can be addressed using the expressions for the Kerr effects associated with the Josephson Ring Modulator

### Beyond third-order expansion: Kerr effect

Higher order non-linearities bring spurious effects.

In particular, the Kerr effect results from the fourth order non-linear term provided by the Josephson Ring Modulator. Remarkably, it does not vanish in the rotating wave approximation (RWA) since only mode populations come into play. The corresponding Hamiltonian is of the form

$$H_{Kerr} = \hbar K_{aa}(a^\dagger a)^2 + \hbar K_{mm}(m^\dagger m)^2 + \hbar K_{am}a^\dagger a m^\dagger m + \hbar K_{ap}|p|^2 a^\dagger a + \hbar K_{mp}|p|^2 m^\dagger m \quad (S22)$$

Two types of terms appear, self-Kerr terms that involve only one mode to the fourth power and cross-Kerr terms that couple the populations of two modes. The self-Kerr effect induces anharmonicity in the modes whereas the cross-Kerr effect induces a linear shift of the resonance frequency of one mode depending on the population of the other mode.

The Kerr terms can be easily derived from the Josephson Hamiltonian involving fourth order of field operators. Hence starting from the ring Hamiltonian, we get

$$\begin{aligned} H_{Kerr} &= -\frac{E_J}{16} \cos \frac{\varphi}{4} \left[ \varphi_a^2 \varphi_m^2 + \varphi_a^2 \varphi_p^2 + \varphi_m^2 \varphi_p^2 + \frac{\varphi_a^4}{24} + \frac{\varphi_m^4}{24} \right] \\ &= -\frac{\cos \varphi/4}{16 L_J^0 \varphi_0^2} \left[ \frac{\hbar^2}{4} Z_a Z_m \xi_a^2 \xi_b^2 a^\dagger a b^\dagger b + \frac{\hbar}{2} Z_a \xi_a^2 \varphi_p^2 a^\dagger a + \frac{\hbar}{2} Z_m \xi_b^2 \varphi_p^2 m^\dagger m \right. \\ &\quad \left. + \frac{\hbar^2}{96} Z_a^2 \xi_a^4 (a^\dagger a)^2 + \frac{\hbar^2}{96} Z_m^2 \xi_m^4 (m^\dagger m)^2 \right] \end{aligned} \quad (S23)$$

The frequency shifts due to the pump tone read

$$\begin{aligned} K_{ap}|p|^2 &= -\frac{1}{32} \omega_a \xi_a |\varphi_p|^2 \frac{L_{JRM}(\varphi_{ext})}{L_J(\varphi_{ext})} \\ K_{mp}|p|^2 &= -\frac{1}{32} \omega_m \xi_m |\varphi_p|^2 \frac{L_{JRM}(\varphi_{ext})}{L_J(\varphi_{ext})} \end{aligned} \quad (S24)$$

In a way, these terms are harmless if the pump amplitude is kept constant. Indeed, they corresponds to a renormalization of the resonance frequency.

The Kerr terms between  $a$  and  $m$  read

$$\begin{aligned} K_{am} &= -\frac{1}{64} \sqrt{\xi_a^5 \omega_a \frac{Z_a}{Z_Q}} \sqrt{\xi_b^5 \omega_b \frac{Z_m}{Z_Q}} \frac{L_{JRM}(\varphi_{ext})}{L_J(\varphi_{ext})} \\ K_{aa} &= -\frac{1}{1536} \xi_a^5 \omega_a \frac{Z_a}{Z_Q} \frac{L_{JRM}(\varphi_{ext})}{L_J(\varphi_{ext})} \\ K_{mm} &= -\frac{1}{1536} \xi_m^5 \omega_m \frac{Z_m}{Z_Q} \frac{L_{JRM}(\varphi_{ext})}{L_J(\varphi_{ext})} \end{aligned} \quad (S25)$$

Note that the self-Kerr terms are much weaker than the cross-Kerr terms.

### Measured Kerr effects

Importantly, the cross-Kerr effects involving the pump are dominant here. Indeed, we are probing the resonators at low photon number ( $\sim 100$ ), thus the self-Kerr terms  $(a^\dagger a)^2$  and  $(m^\dagger m)^2$  as well as the cross-Kerr term  $a^\dagger a m^\dagger m$

are negligible compared to the cross-Kerr involving the pump that is strongly driven. The correction to the resonance frequencies of mode  $a$  at rest is given by

$$\begin{aligned} K_{ap}|p|^2 &= \frac{1}{32L_J^0} \cos \frac{\varphi}{4} Z_a \xi_a^2 |\varphi_p|^2 \\ &= \frac{1}{32} \omega_a \xi_a |\varphi_p|^2 \end{aligned} \quad (\text{S26})$$

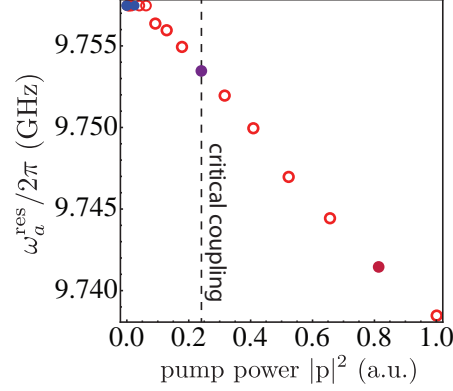

Figure S4: Measured buffer resonance frequency as a function of pump power  $|p|^2$  in arbitrary unit (in the cool down corresponding to Fig. 2 in the main text). The largest displayed pump power corresponds to the one used for catch and release in Fig. 2. Note that the measurements performed during the second cool down at a different flux bias (for Figs 3 and 4 of the main text) were taken with even larger Kerr nonlinearities.

As derived in the previous section, the strong coupling regime is reached for

$$\chi|p| = \frac{\varphi_p}{2} \sin \frac{\varphi_{ext}}{4} \sqrt{\xi_a \xi_m \omega_a \omega_m} \sim \frac{\kappa_a}{2} \quad (\text{S27})$$

Therefore, the frequency shift of the buffer mode induced by the pump in the strong coupling regime reads

$$K_{ap}|p|^2 \sim \frac{1}{(\tan \frac{\varphi}{4})^2} \frac{\kappa_a^2}{2\xi_m \omega_m} \sim \frac{\kappa_a}{\xi_m Q_a} \approx 2\pi \times 20 \text{ MHz} \quad (\text{S28})$$

Similarly, the frequency shift induced by the pump on the memory mode  $m$  can be estimated to

$$K_{mp}|p|^2 \sim \frac{\kappa_m}{\xi_a Q_m} < 2\pi \times 1 \text{ kHz} \quad (\text{S29})$$

Similarly to what is observed in the experiment, the Kerr frequency shift is negligible on the memory cavity.

The estimated value of the Kerr frequency shift is in good agreement with the one measured on the buffer mode  $a$  and presented in S4. We observe a linear dependence with pump power and a shift of 20 MHz for the largest pump powers in the strong coupling regime, which is the one used for Fig. 2 in the main text.

## QUANTUM LANGEVIN EQUATION

The quantum Langevin equation offers a convenient framework to study the interplay between the memory mode  $m$ , the buffer mode  $a$  and the propagating mode  $a_{in}$  and  $a_{out}$  as a function of the pump amplitude  $p$ .

The quantum Langevin equation gives the evolution of electromagnetic modes coupled to propagating modes.

$$\begin{cases} \frac{\partial a}{\partial t} = \frac{i}{\hbar}[H, a] - \frac{\kappa_a}{2}a + \sqrt{\kappa_a}a_{in} \\ \frac{\partial m}{\partial t} = \frac{i}{\hbar}[H, m] - \frac{\kappa_m}{2}m + \sqrt{\kappa_m}m_{in} \end{cases} \quad (S30)$$

In the conversion mode, the system Hamiltonian in the rotating wave approximation ( $\omega_p = \omega_a - \omega_m$ ) reads

$$H = \hbar\omega_a^{\text{res}}a^\dagger a + \hbar\omega_m^{\text{res}}m^\dagger m + \hbar\chi(p a^\dagger m + p^* a m^\dagger) \quad (S31)$$

The interaction Hamiltonian couples linearly the two Langevin equation

$$\begin{cases} \frac{\partial a}{\partial t} = -i\omega_a^{\text{res}}a - i\chi p m - \frac{\kappa_a}{2}a + \sqrt{\kappa_a}a_{in} \\ \frac{\partial m}{\partial t} = -i\omega_m^{\text{res}}m - i\chi p^* a - \frac{\kappa_m}{2}m + \sqrt{\kappa_m}m_{in} \end{cases} \quad (S32)$$

Here, as in the experiment we will discuss, we consider only a constant pump amplitude. Note that the following expressions need to be modified in case of a varying pump amplitude.

One can write the Langevin equation in the frequency domain knowing that  $p(t) = p_0 e^{-i\omega_p t}$  considering that  $\omega_p = \omega_a^{\text{res}} - \omega_m^{\text{res}}$

$$\begin{cases} 0 = i(\omega_a - \omega_a^{\text{res}} + i\frac{\kappa_a}{2})a[\omega_a] - i\chi p_0 m[\omega_m] + \sqrt{\kappa_a}a_{in}[\omega_a] \\ 0 = i(\omega_m - \omega_m^{\text{res}} + i\frac{\kappa_m}{2})m[\omega_m] - i\chi p_0^* a[\omega_a] + \sqrt{\kappa_m}m_{in}[\omega_m] \end{cases} \quad (S33)$$

From this equation, we can derive the quantum scattering relation between the input mode  $a_{in}$  and  $m_{in}$  and the cavity modes  $m$  and  $a$ .

$$m[\omega_m] = \frac{i(\chi p_0)^* \sqrt{\kappa_a}}{(\omega_m - \omega_m^{\text{res}} + i\kappa_m/2)(\omega_a - \omega_a^{\text{res}} + i\kappa_a/2) - |\chi p_0|^2} a_{in}[\omega_a] + \frac{i\sqrt{\kappa_m}(\omega_a - \omega_a^{\text{res}} + i\kappa_a/2)}{(\omega_m - \omega_m^{\text{res}} + i\kappa_m/2)(\omega_a - \omega_a^{\text{res}} + i\kappa_a/2) - |\chi p_0|^2} m_{in}[\omega_m] \quad (S34)$$

$$a[\omega_a] = \frac{i\sqrt{\kappa_a}(\omega_m - \omega_m^{\text{res}} + i\kappa_m/2)}{(\omega_m - \omega_m^{\text{res}} + i\kappa_m/2)(\omega_a - \omega_a^{\text{res}} + i\kappa_a/2) - |\chi p_0|^2} a_{in}[\omega_a] + \frac{i(\chi p_0)^* \sqrt{\kappa_a}}{(\omega_m - \omega_m^{\text{res}} + i\kappa_m/2)(\omega_a - \omega_a^{\text{res}} + i\kappa_a/2) - |\chi p_0|^2} m_{in}[\omega_a] \quad (S35)$$

We now define  $\Delta = \omega_a - \omega_a^{\text{res}} = \omega_m - \omega_m^{\text{res}}$  and we can eliminate the buffer mode  $a$  from these equations using the input/output relation  $\sqrt{\kappa_a}a = a_{in} + a_{out}$

### Amplitude scattering coefficient

The losses of mode  $m$  can be modeled as propagating modes  $m_{in/out}$  evolving on an uncontrolled port then  $\langle m_{in}[\omega_m] \rangle = 0$ . Thus, the scattering coefficients read

$$\begin{aligned} \langle m[\omega_m] \rangle &= \frac{i\chi p_0^* \sqrt{\kappa_a}}{(\Delta + i\kappa_m/2)(\Delta + i\kappa_a/2) - |\chi p_0|^2} \langle a_{in}[\omega_a] \rangle \\ \langle m[\omega_m] \rangle &= \frac{-i\chi p_0^* \sqrt{\kappa_a}}{(\Delta + i\kappa_m/2)(\Delta - i\kappa_a/2) - |\chi p_0|^2} \langle a_{out}[\omega_a] \rangle \\ \langle a_{out}[\omega_a] \rangle &= -\frac{(\Delta + i\kappa_m/2)(\Delta - i\kappa_a/2) - |\chi p_0|^2}{(\Delta + i\kappa_m/2)(\Delta + i\kappa_a/2) - |\chi p_0|^2} \langle a_{in}[\omega_a] \rangle \end{aligned} \quad (S36)$$

We can rewrite these equations such that the denominators are put under a factorized form.

$$\begin{aligned} \langle m[\omega_m] \rangle &= \frac{-4\chi p_0^* \sqrt{\kappa_a}}{(\gamma_i^a - 2i\Delta)(\gamma_i^m - 2i\Delta)} \langle a_{in}[\omega_a] \rangle \\ \langle m[\omega_m] \rangle &= \frac{-4\chi p_0^* \sqrt{\kappa_a}}{(\gamma_o^a + 2i\Delta)(\gamma_o^m + 2i\Delta)} \langle a_{out}[\omega_a] \rangle \\ \langle a_{out}[\omega_a] \rangle &= -\frac{(\gamma_o^a + 2i\Delta)(\gamma_o^m + 2i\Delta)}{(\gamma_i^a - 2i\Delta)(\gamma_i^m - 2i\Delta)} \langle a_{in}[\omega_a] \rangle \end{aligned} \quad (S37)$$

Therefore, poles of the scattering coefficient are given by  $\pm i\gamma_{i/o}^{a/m}/2$ . The  $i/o$  labeling depends on whether the scattering coefficient couples  $\langle m \rangle$  to  $\langle a_{in} \rangle$  or  $\langle a_{out} \rangle$ . The  $a/m$  labeling refers to the zero pump limit,  $\gamma_{i/o}^a \rightarrow \kappa_a$  and  $\gamma_{i/o}^m \rightarrow \pm \kappa_m$ . This labeling will become clear when the temporal evolution of the fields will be considered.

Actually, the dynamical coupling rates between the propagating modes  $a_{in}$  and  $a_{out}$  and the memory mode  $m$ , which occur through the buffer, is defined as

$$\gamma_i^m = \frac{\kappa_a + \kappa_m}{2} - \sqrt{\left(\frac{\kappa_a - \kappa_m}{2}\right)^2 - 4|\chi p_0|^2} \quad (\text{S38})$$

and

$$\gamma_o^m = \frac{\kappa_a - \kappa_m}{2} - \sqrt{\left(\frac{\kappa_a + \kappa_m}{2}\right)^2 - 4|\chi p_0|^2} \quad (\text{S39})$$

Similarly, the dynamical coupling rates between the propagating modes  $a_{in}$  and  $a_{out}$  and the buffer mode  $a$  are defined as

$$\gamma_i^a = \frac{\kappa_a + \kappa_m}{2} + \sqrt{\left(\frac{\kappa_a - \kappa_m}{2}\right)^2 - 4|\chi p_0|^2} \quad (\text{S40})$$

and

$$\gamma_o^a = \frac{\kappa_a - \kappa_m}{2} + \sqrt{\left(\frac{\kappa_a + \kappa_m}{2}\right)^2 - 4|\chi p_0|^2} \quad (\text{S41})$$

### DYNAMICAL COUPLING RATES

In the limit of a long-lived memory  $\kappa_a \gg \kappa_m$ , we can define the input/output coupling rate to the memory

$$\boxed{\gamma_{io}^m = \frac{\kappa_a}{2} \left[ 1 - \sqrt{1 - 16 \frac{|\chi p_0|^2}{\kappa_a^2}} \right]} \quad (\text{S42})$$

such that[8]

$$\begin{aligned} \gamma_i^m &\approx \gamma_{io}^m + \kappa_m \\ \gamma_o^m &\approx \gamma_{io}^m - \kappa_m \end{aligned} \quad (\text{S43})$$

Besides, the input/output coupling rate to the buffer can be defined

$$\gamma_{io}^a = \frac{\kappa_a}{2} \left[ 1 + \sqrt{1 - 16 \frac{|\chi p_0|^2}{\kappa_a^2}} \right] \quad (\text{S44})$$

such that

$$\boxed{\gamma_{io}^a = \kappa_a - \gamma_{io}^m \approx \gamma_i^a \approx \gamma_o^a} \quad (\text{S45})$$

### Limits on the coupling rates

We can decompose the two limits on the coupling rates

- For weak pump tone the coupling increases linearly with pump power

$$\gamma_{io}^m(|\chi p_0| \ll \kappa_a) = \frac{4|\chi p_0|^2}{\kappa_a} \quad (\text{S46})$$

- For stronger pump tone  $|\chi p_0| > \kappa_a/4$ , the system enters in the strong regime limit. The coupling rate  $\chi p_0$  exceeds the buffer exit rate  $\kappa_a/2$ , thus the two modes hybridize. The dynamical coupling rate becomes complex. Its real part defines the effective coupling rate. It saturates to half the buffer escape rate

$$\gamma_{io}^m(|\chi p_0| > \kappa_a/4) = \frac{\kappa_a}{2} \quad (\text{S47})$$

Its imaginary part corresponds to the dispersive shift of resonance frequencies.

$$\delta\omega_{\pm}^m(|\chi p_0| > \kappa_a/4) = \text{Im}(\gamma_{io}^{a/m}/2) = \pm \sqrt{|\chi p_0|^2 - \left(\frac{\kappa_a}{4}\right)^2} \quad (\text{S48})$$

To put it simply, the conversion rate between modes at frequency  $\omega_a$  and  $\omega_m$  becomes large enough so that, effectively, these two modes hybridize. The new resonant modes are combinations of the buffer and memory modes, despite the frequency detuning between them. The strong coupling induces a splitting between the new resonant modes, whose magnitude scales with the pump amplitude.

### Effect of the antennas

The 3D cavity is capacitively coupled to the Jopsephson Ring Modulator through antennas. This capacitive coupling  $\kappa_c$  placed in series with the conversion coupling  $|\chi p|$ , leads to an effective conversion rate between  $m$  and  $a$  given by

$$|\chi p_0|^2 \leftarrow \frac{1}{\frac{1}{(\kappa_c/2)^2} + \frac{1}{|\chi p_0|^2}} \quad (\text{S49})$$

Hence, the effective coupling rate reads

$$\gamma_{io}^m = \frac{\kappa_a}{2} \left( 1 - \sqrt{1 - \frac{4}{\kappa_a^2 \left( \frac{1}{\kappa_c^2} + \frac{1}{4|\chi p_0|^2} \right)}} \right) \quad (\text{S50})$$

When the conversion rate is small compared to this capacitive coupling, the dynamical coupling is not modified

$$\gamma_{io}^m(|\chi p| \ll \kappa_c) = \frac{4|\chi p|^2}{\kappa_a} \quad (\text{S51})$$

However when the conversion rate overcomes the capacitive coupling, we observe a saturation of the dynamical coupling rate due to the antennas. It is given by

$$\gamma_{io}(|\chi p| \gg \kappa_c) = \frac{\kappa_a}{2} \left( 1 - \sqrt{1 - \left( \frac{2\kappa_c}{\kappa_a} \right)^2} \right) \quad (\text{S52})$$

### DETERMINATION OF THE COUPLING TO THE ANTENNAS

The antenna coupling has been designed and tested with dedicated samples. These samples consisted in capacitive pads directly connected to the input connectors as shown in Fig. S5. At room temperature, the 3D cavity was probed in reflection (Fig. S5b) in a similar way that one would probe in reflection a two port  $\lambda/2$  resonator as the buffer resonator for instance (Fig. S5a). The measured reflection coefficient as a function of the frequency has enabled us to extract the direct coupling rate  $\kappa_c$  between the 50  $\Omega$  microstrip line and the 3D cavity. Various shapes and sizes of capacitive pads has been tested. We have selected the capacitive pads providing a capacitive coupling rate of  $\kappa_c = 3$  MHz. It corresponds to the geometry represented in Fig. S5b and detailed in Fig. S6c.

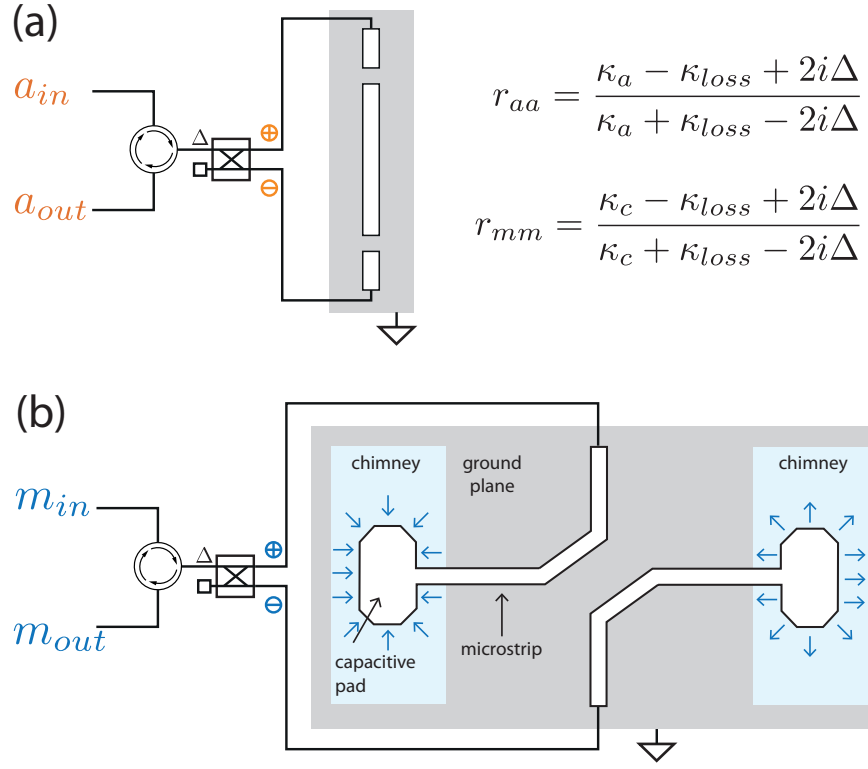

Figure S5: Capacitive couplings calibration (a) Setup for the reflection measurement of two ports  $\lambda/2$  microstrip resonator. (b) Setup for the reflection measurement of the 3D memory cavity for testing the capacitive pads of the antenna.

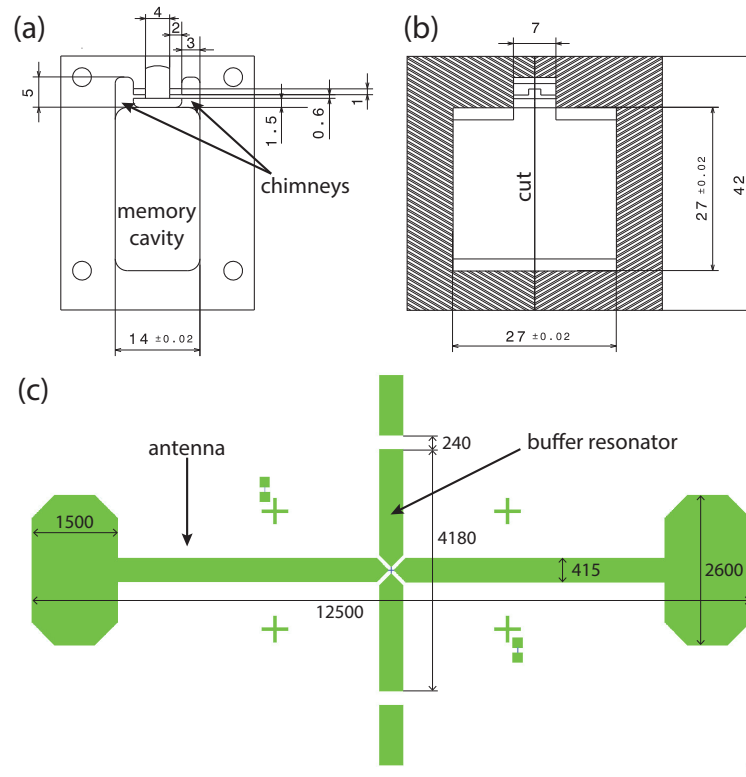

Figure S6: (a) One half of the cavity is shown from the front side (lengths in mm). (b) A section of the two halves of the cavity put together is shown from the side (lengths in mm). The cut is represented as a vertical, thick black line in the center. (c) Drawing of the device used in e-beam lithography (lengths in microns). The two symmetric antennas ending within the chimneys by oval shaped pads are oriented horizontally.

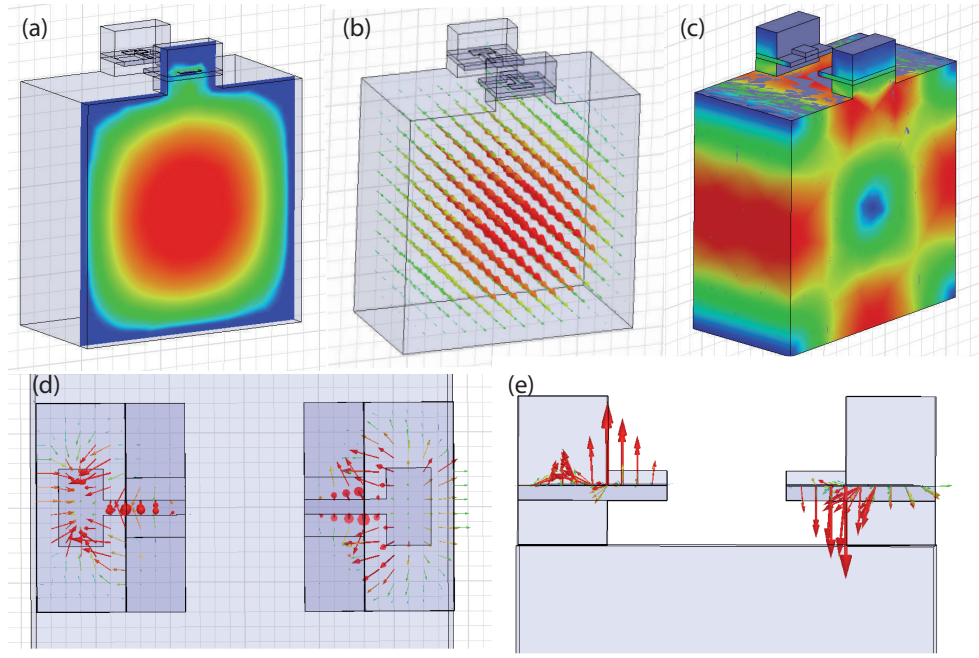

Figure S7: Simulations of the fundamental mode at 7.8 GHz, well separated from the second mode at 13 GHz. (a) Amplitude of the electric field along a section of the cavity crossing the pads of the antenna of the TE<sub>110</sub> mode (blue is zero and red is maximal). (b) Vectorial view of the TE<sub>110</sub> mode. (c) Current intensity along the surface of the cavity. (d) (e) Coupling of the TE<sub>110</sub> mode to the capacitive pads, electric field at the surface of the substrate.

## TIME-CONTROLLED STORAGE AND RETRIEVAL

In a practical quantum network architecture, the quantum memory of each node must be able to store, process and exchange a quantum field in a time-controlled way. The temporal shape of the transmitted fields plays a crucial role in the efficiency of each node. Indeed, the temporal envelope of the field released by the sender memory must be adjusted to be efficiently captured by the receiver memory. For a finite memory bandwidth, the optimal temporal shape is symmetric by time reversal [? ].

In principle in our device, it is possible to generate and capture time symmetric pulses by properly adjusting the pump amplitude in time. However, due to the Kerr effect discussed in section , finding the optimal pump temporal shape is a difficult problem. In what follows, we thus focus on the dual approach in which the temporal shape of an incoming coherent state is optimized so that it is most efficiently captured by a square pump pulse.

Let us first consider a sequence in which the memory records an incoming pulse before time 0 and then keep it stored. The corresponding pump amplitude remains constant at  $t < 0$  and zero for  $t > 0$ , so that the input/output rate is given by  $\gamma_{io}(t) = \gamma_0\theta(-t)$  where  $\theta$  is the Heaviside function. The incoming pulse, sent before time 0 propagates on the transmission line towards the memory while the pump is on so that  $\langle a_{in}(t) \rangle = f_{in}(t)\theta(-t)$ . What is the temporal shape of this wave packet that maximizes the efficiency of its capture by the memory?

Here, by efficient, we mean that the memory keeps as much of the incoming energy as possible without releasing it. This corresponds to requesting that  $\langle a_{out}(t) \rangle = 0$  at all times when the pump amplitude ensures that  $\gamma_{io}(t) = \gamma_0\theta(-t)$ . Given that the incoming pulse stops at time 0, this condition is met for  $t > 0$  as long as the buffer mode  $a$  stays empty, which leads to

$$\begin{cases} \langle a_{out}(t) \rangle = 0 & \text{for } t < 0 \\ \langle a(t=0) \rangle = 0 \end{cases} \quad (\text{S53})$$

This criterion depends on negative times only so that its solutions  $\langle a_{in}(t) \rangle = f_{in}(t)\theta(-t)$  can be found by considering a constant coupling  $\gamma_{io}(t) = \gamma_0$  even at positive times.

### Absorption without reflection

Let us first note that the poles of the Fourier transform of  $\langle a_{in}(t) \rangle$  are all in the upper-half plane of the complex plane since it is non-zero only for  $t < 0$ . Moreover, the first line of Eq. (S53) imposes that  $\langle a_{out}(t) \rangle$  must be zero for  $t < 0$ , thus the poles of its Fourier transform must all be in the lower-half plane of the complex plane.

This stringent condition can be satisfied since the reflection coefficient relating  $a_{out}$  to  $a_{in}$  input and output has poles and zeros that are perfectly fit for transforming poles of the upper-half plane into poles of the lower-half plane. Indeed, for large coupling rates  $\gamma_{io}^m \gg \kappa_m$ , the reflection coefficient reads

$$\langle a_{out}[\omega_a] \rangle = -\frac{(\kappa_a - \gamma_{io}^m + 2i\Delta)(\gamma_{io}^m + 2i\Delta)}{(\kappa_a - \gamma_{io}^m - 2i\Delta)(\gamma_{io}^m - 2i\Delta)} \langle a_{in}[\omega_a] \rangle \quad (\text{S54})$$

By choosing the poles of the input signal  $\langle a_{in}[\omega_a] \rangle$  to coincide with the zeros of the scattering coefficient, one gets an output field  $\langle a_{out}[\omega_a] \rangle$  with poles in the lower half-plane only as requested.

Therefore, the optimal input signal is of the form

$$\langle a_{in}[\omega_a] \rangle = \frac{\alpha}{\gamma_{io}^m + 2i\Delta} + \frac{\beta}{\kappa_a - \gamma_{io}^m + 2i\Delta} \quad (\text{S55})$$

and leads to an output signal equal to

$$\langle a_{out}[\omega_a] \rangle = -\alpha \frac{\kappa_a - \gamma_{io}^m + 2i\Delta}{(\kappa_a - \gamma_{io}^m - 2i\Delta)(\gamma_{io}^m - 2i\Delta)} \quad (\text{S56})$$

$$-\beta \frac{\gamma_{io}^m + 2i\Delta}{(\kappa_a - \gamma_{io}^m - 2i\Delta)(\gamma_{io}^m + \kappa_m - 2i\Delta)} \quad (\text{S57})$$

In the time domain, the input field corresponds to an increasing exponential of the form

$$\langle a_{in}(t) \rangle = \alpha\theta(-t)e^{\frac{\gamma_{io}^m}{2}t} + \beta\theta(-t)e^{\frac{\kappa_a - \gamma_{io}^m}{2}t} \quad (\text{S58})$$

Qualitatively, the first term is mostly absorbed by the memory at a rate  $\gamma_{io}^m$  and the second term is mostly absorbed by the buffer at the  $\gamma_{io}^b = \kappa_a - \gamma_{io}^m$ . Up to now, we have not considered the second line in Eq. (S53), which ensures that a complete transfer to the memory has been performed. One must then find the right balance between  $\alpha$  and  $\beta$  to verify  $\langle a(t=0) \rangle = 0$ .

### Complete transfer

For a complete transfer, one must be sure that no fields remain in the buffer at  $t = 0$  when the coupling is turned off. This constraint imposes that

$$\langle a(t=0) \rangle = \int_{-\infty}^{+\infty} \langle a[\omega_a] \rangle d\omega_a = 0. \quad (\text{S59})$$

leading to

$$\kappa^{-1/2} \int_{-\infty}^{+\infty} \langle a_{in}[\omega_a] \rangle + \langle a_{out}[\omega_a] \rangle d\omega_a = 0. \quad (\text{S60})$$

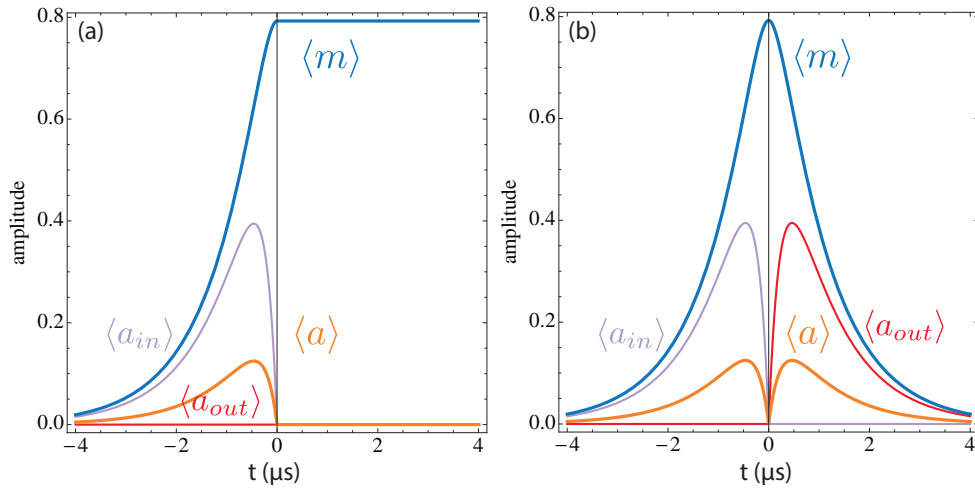

Figure S8: (a) Expected time dependence of the various mode amplitudes for the optimal temporal shape of the input field  $\langle a_{in} \rangle$  and a pump amplitude turned off at time 0 so that  $\gamma_{io}^m = \theta(-t) \times 2 \mu\text{s}^{-1}$ . Here, we assume  $\kappa_a = 10 \mu\text{s}^{-1}$  and  $\kappa_m = 0$ . (b) Same curves when the pump is kept on so that  $\gamma_{io}^m = 2 \mu\text{s}^{-1}$ .

This condition is met when  $\alpha = -\beta$ . Hence the optimally absorbed input fields reads

$$\langle a_{in}[\omega_a] \rangle \propto \frac{1}{\kappa_a/2 - \gamma_{io}^m} \left( \frac{1}{\gamma_{io}^m + 2i\Delta} - \frac{1}{\kappa_a - \gamma_{io}^m + 2i\Delta} \right) \quad (\text{S61})$$

$$\propto \frac{1}{(\gamma_{io}^m - \kappa_m + 2i\Delta)(\kappa_a - \gamma_{io}^m + 2i\Delta)} \quad (\text{S62})$$

and leads to an output field

$$\langle a_{out}[\omega_a] \rangle \propto \frac{-1}{\kappa_a/2 - \gamma_{io}^m} \left( \frac{1}{\gamma_{io}^m - 2i\Delta} - \frac{1}{\kappa_a - \gamma_{io}^m - 2i\Delta} \right) \quad (\text{S63})$$

$$\propto \frac{-1}{(\gamma_{io}^m - \kappa_m - 2i\Delta)(\kappa_a - \gamma_{io}^m - 2i\Delta)} \quad (\text{S64})$$

We can now give the expressions of the optimally caught input signal in the time domain (see Fig. S8)

$$\langle a_{in}(t) \rangle \propto \theta(-t) \left( e^{\frac{\gamma_{io}^m}{2} t} - e^{\frac{\kappa_a - \gamma_{io}^m}{2} t} \right) \quad (\text{S65})$$

The first term ensures absorption without reflection, while the second term permits the complete transfer of the absorbed pulse from the buffer to the memory cavity. It is worth to note that the optimally captured signal is simply the time-reverse of a signal retrieved from an initially occupied memory. This retrieved signal can be observed experimentally on  $a_{out}$  by preparing the memory in a coherent state with the pump off, and then turning it on (or on Fig. S8b at  $t > 0$ ).

With this signal shape at the input, no signal is reflected and  $\langle a_{out}(t) \rangle = 0$  if the pump is turned off at time 0, and the field is stored in the memory mode  $m$  (see Fig. S8a). However, if the pump remains on at all times, the output field is given by (see Fig. S8b)

$$\langle a_{out}(t) \rangle \propto \theta(t) \left( e^{-\frac{\gamma_{io}^m}{2} t} - e^{-\frac{\kappa_a - \gamma_{io}^m}{2} t} \right) \quad (\text{S66})$$

Finally, in the special case of the strong coupling regime for which  $\gamma_{io}^m = \kappa_a/2$ , the above expression breaks down and the optimal signals are given by

$$\langle a_{in}(t) \rangle \propto \theta(-t) t e^{\kappa_a t/2} \quad (\text{S67})$$

$$\langle a_{out}(t) \rangle \propto \theta(t) t e^{-\kappa_a t/2} \quad (\text{S68})$$

## MEASUREMENT OF THE AMPLITUDE GAIN

In the experiment entanglement is generated between the memory and a propagating mode by sending a square pump pulse at frequency  $f_a + f_m$  with an initially empty memory. If the memory is initially occupied by a coherent state, the same pulse will result in parametric amplification. It was necessary to properly calibrate the gain of this amplification to determine the entanglement threshold in the experiment. Since, the pump is not continuous, we have developed a protocol to perform an accurate measurement of this pulsed amplitude gain.

First, we capture a coherent state in the quantum memory by turning the pump tone at the difference frequency  $f_a - f_m$ . Then we turn on the entanglement pulse by applying a pump at the sum frequency  $f_a + f_m$ . It provides a direct amplitude gain  $\sqrt{G} = \cosh(r)$  on the memory mode  $\hat{m}$  and a cross amplitude gain  $\sqrt{G-1} = \sinh(r)$  from the memory mode  $\hat{m}$  to the transmission line mode  $\hat{a}_{out}$ . Finally we retrieve the amplified captured state in the transmission line by turning on the pump tone at the difference frequency again.

We can repeat this measurement without the entanglement pulse, thus the amplitude gain is turn off,  $\sqrt{G} = \cosh(0) = 1$ .

The ON/OFF ratio of the squared integrated amplitude of the retrieval pulse provides the gain  $G = \cosh^2(r)$ . This protocol enables to determine the gain independently of the losses due to the inefficiency of the device.

As shown in Figure S9, we repeat this measurement for an increasing incoming wave packet energy. The amplification process is linear on this energy scale, and it is important to check that the device is not saturated. The ratio of the slopes gives a gain  $G = \cosh^2(r) = 2.29$ .

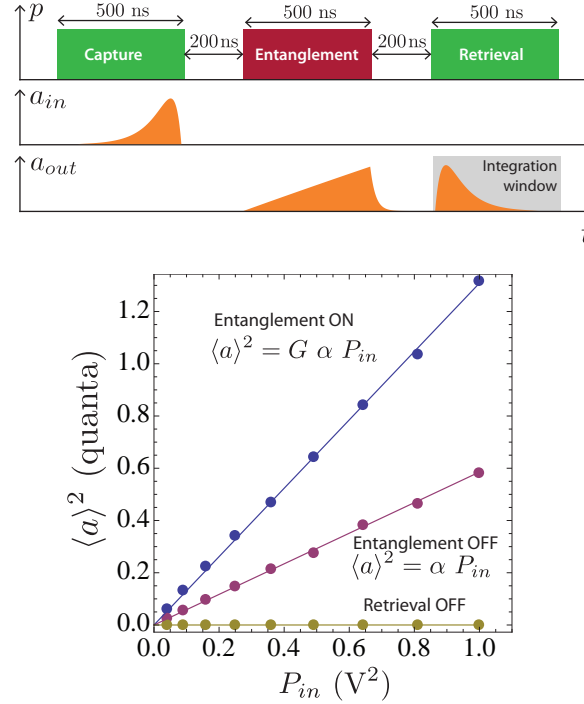

Figure S9: Amplitude gain measurement protocol. The upper panel presents the timing of the pulsed measurement. The lower panel presents the measurement results. It gives the squared amplitude of the retrieved field as a function of the power of the source that generates the captured wave (square of the modulation amplitude). The squared amplitude gain is given by the ratio of the slopes.

## PHASE LOCKING

In this section, we stress that the relative phases of the local oscillators must be carefully locked in our experiment. As shown in Fig.S10, various frequencies are implied in the conversion and entanglement processes.

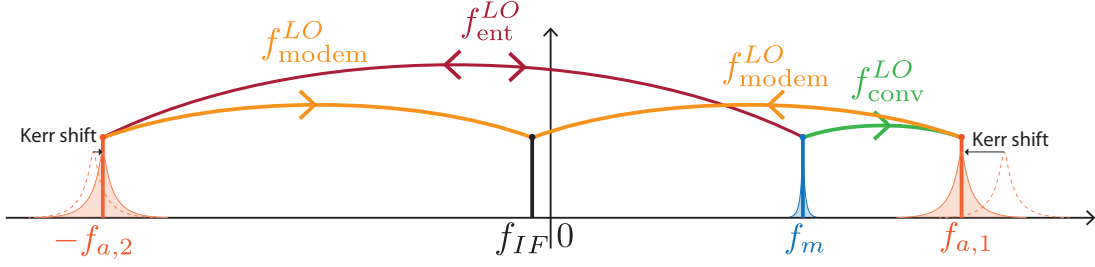

Figure S10: Schematics of the frequency relations between the local oscillators. In practice, the local oscillators frequencies are  $f_{ent}^{LO} = 17.28625$  GHz,  $f_{conv}^{LO} = 1.6575$  GHz and  $f_{modem}^{LO} = 9.471875$  GHz, the intermediate frequency is  $f_{IF} = 25.5$  MHz and the mode frequencies are  $f_m = 7.78888$  GHz,  $f_{a,1} = 9.44638$  GHz,  $f_{a,2} = 9.49738$  GHz

For instance when an entangled state is generated, it is shared between the memory at a positive frequency  $f_m$  and the buffer at a negative frequency  $-f_{a,2}$ . Phase locking is provided by the local oscillator at  $f_{ent}^{LO} = f_m + f_{a,2}$  producing the entanglement.

On the one hand, the part of the state that propagates at  $-f_{a,2}$  gets down-converted at the intermediate frequency (IF) for readout by the demodulation local oscillator ( $f_{modem}^{LO}$ ) on the negative side such that  $f_{IF} = f_{modem}^{LO} - f_{a,2}$  (see Fig.S10).

On the other hand, the part of the state stored in the cavity at  $f_m$  is retrieved in the transmission line by the conversion local oscillator ( $f_{conv}^{LO}$ ) at the buffer frequency  $f_{a,1} = f_m + f_{conv}^{LO}$ . Then the signal is downconverted at the intermediate frequency IF by the same demodulation local oscillator such that  $f_{IF} = f_{modem}^{LO} - f_{a,1}$ . Note that  $f_{a,1}$  differs from  $f_{a,2}$  due to Kerr effect with different pump powers (see section on Kerr effect).

In the end, all the local oscillator frequencies are locked by the relation  $f_{ent}^{LO} + f_{conv}^{LO} = 2f_{modem}^{LO}$ . As a consequence, the experiment requires a relative phase stability of these three local oscillators greater than the total acquisition time of the order of 5 min. We have reached such a phase stability by carefully synchronizing our three commercial sources (Agilent E8257D) using their 10 MHz synchronization port and rigid coaxial cables.

Note that in usual spectral measurement, the phase stability of local oscillator is not as crucial as here, the signal is up-converted and down-converted by the same local oscillator then the phases cancel out. Here, the measurement sequence presented in Fig.S10 consists in up-converting a signal from IF to  $f_{a,1}$  then store it at  $f_m$ , amplifying it at  $-f_{a,2}$  and finally down-converting the signal at IF. In this sequence, the phases of the local oscillators accumulate instead of canceling out.

## NOISE CALIBRATION

### Measurement outcome probability distribution

During the entanglement step, the Josephson Ring Modulator performs a reversible transform of the wavefunction of the field via the unitary two-mode squeeze operator  $S = \exp(re^{i\varphi_P} a^\dagger m^\dagger - re^{-i\varphi_P} am)$  where  $re^{i\varphi_P}$  is the complex squeezing parameter, and  $a$  and  $m$  are the field operators of the two modes [4]. The input and output canonical field operators are related by the scattering relations

$$a_{out,1} = S^\dagger a_{in} S = \cosh(r) a_{in} + e^{i\varphi_P} \sinh(r) m_{in,1}^\dagger, \quad (S69)$$

where  $\varphi_P$  is the phase of the pump and  $G = \cosh^2 r$  is the power direct gain which increases with pump power  $|p|^2$ . With the pump on, the vacuum state at the input is converted into a two-mode squeezed vacuum state  $|Sq\rangle = S|0\rangle_a|0\rangle_m = \cosh(r)^{-1} \sum \tanh(r)^n |n\rangle_a |n\rangle_m$ .

In a second step, after a delay time  $\tau$ , we apply the retrieval pulse to transfer the  $m$  mode in the transmission line mode  $a_{out}$  with an efficiency  $\eta$ . The outgoing mode produced during the entanglement step is denoted by  $a_{out,1}$  while the one associated with the retrieval after a time  $\tau$  is denoted by  $a_{out,2}$ . The finite efficiency  $\eta$  may be modeled by the contribution of a mode  $m_{in,2}$ , uncorrelated with all other modes.

$$a_{out,2} = \sqrt{\eta} S^\dagger m_{in,1} S + \sqrt{1-\eta} m_{in,2} = \sqrt{\eta} [\cosh(r) m_{in,1} + e^{-i\varphi_P} \sinh(r) a_{in}^\dagger] + \sqrt{1-\eta} m_{in,2} \quad (S70)$$

$$(S71)$$

The output signal  $a_{out}$  is then amplified by a noisy amplifying setup with a gain  $G_{amp}$ . The uncorrelated noise added by the amplifying setup is modeled by the bosonic operator  $h_{in}$  whose effective temperature is mainly determined by the noise temperatures of the cold HEMT amplifier. Thus, we collect the measurement outcomes of the operator  $A_{out}$  and  $M_{out}$ .

$$A_{out} = \sqrt{G_{amp}} a_{out,1} + \sqrt{G_{amp} - 1} h_{1,in}^\dagger \quad (S72)$$

$$= \sqrt{G_{amp}} (\cosh(r) a_{in} + e^{i\varphi_P} \sinh(r) m_{in,1}^\dagger) + \sqrt{G_{amp} - 1} h_{2,in}^\dagger \quad (S73)$$

$$M_{out} = \sqrt{G_{amp}} a_{out,2} + \sqrt{G_{amp} - 1} h_{2,in}^{2\dagger} \quad (S74)$$

$$= \sqrt{G_{amp}} (\sqrt{\eta} [\cosh(r) m_{in,1} + e^{-i\varphi_P} \sinh(r) a_{in}^\dagger] + \sqrt{1-\eta} m_{in,2}) + \sqrt{G_{amp} - 1} h_{2,in}^\dagger \quad (S75)$$

In order to perform a tomography of the entangled state, we perform a fast digital heterodyne measurement of  $A_{out}$  and  $M_{out}$ . The entanglement and retrieval sequence described in the main text is repeated  $4 \times 10^7$  times. The measurement outcomes are sorted in real-time by the FPGA board. Indeed, the FPGA generates six histograms giving the probability distribution of measurement outcomes as a function of every pair of mode quadratures. The probability distribution measured with an heterodyne detection correspond to  $Q(\alpha, \mu)$  the Q-function of  $(A_{out}, M_{out})$  [5]. The Q-function gives access to the normally ordered moment of the field operators.

$$\langle A_{out}^{p_a} M_{out}^{p_m} A_{out}^{\dagger q_a} M_{out}^{\dagger q_m} \rangle = \int \alpha^{p_a} \mu^{p_m} (\alpha^*)^{q_a} (\mu^*)^{q_m} Q(\alpha, \mu) d^2\alpha d^2\mu. \quad (S76)$$

### Covariance matrix

For simplicity, we identify  $a \equiv a_{out,1}$  (since  $a_{out,1}$  corresponds to what was directly produced on mode  $a$ ) and  $m \equiv a_{out,2}$  (since  $a_{out,2}$  comes from what was stored in the memory). Without loss of generality, we also assume that the mean value of the field operators are zero  $\langle a \rangle = \langle m \rangle = 0$ .

One can calculate the covariance matrix  $\mathcal{V}$  of the two mode state (Fig. S11c), which fully characterizes the EPR state since it is Gaussian with zero mean [6]. In a coordinate system where  $\mathbf{x} = \{\hat{X}_a, \hat{P}_a, \hat{X}_m, \hat{P}_m\}$ , one defines  $\mathcal{V}_{ij} = 4 \left[ \frac{1}{2} \langle x_i x_j + x_j x_i \rangle - \langle x_i \rangle \langle x_j \rangle \right]$ . With this convention, the covariance matrix of the vacuum state is the unity matrix  $\mathbb{I}_4$ .

$$\mathcal{V} = \frac{1}{2} \begin{pmatrix} 2\langle(a+a^\dagger)^2\rangle & -i\langle\{a+a^\dagger, a-a^\dagger\}\rangle & \langle\{a+a^\dagger, m+m^\dagger\}\rangle & -i\langle\{a+a^\dagger, m-m^\dagger\}\rangle \\ -i\langle\{a+a^\dagger, a-a^\dagger\}\rangle & -2\langle(a-a^\dagger)^2\rangle & -i\langle\{a-a^\dagger, m+m^\dagger\}\rangle & -\langle\{a-a^\dagger, m-m^\dagger\}\rangle \\ \langle\{a+a^\dagger, m+m^\dagger\}\rangle & -i\langle\{a-a^\dagger, m+m^\dagger\}\rangle & 2\langle(m+m^\dagger)^2\rangle & -i\langle(m+m^\dagger, m-m^\dagger)\rangle \\ -i\langle\{a+a^\dagger, m-m^\dagger\}\rangle & -\langle\{a-a^\dagger, m-m^\dagger\}\rangle & -i\langle\{m+m^\dagger, m-m^\dagger\}\rangle & -2\langle(m-m^\dagger)^2\rangle \end{pmatrix}. \quad (\text{S77})$$

We expand the field operators in the normal order

$$\mathcal{V} = \begin{pmatrix} \langle a^2 \rangle + \langle a^{\dagger 2} \rangle + 2\langle aa^\dagger \rangle & -i\langle a^2 \rangle - i\langle a^{\dagger 2} \rangle & \langle am \rangle + \langle a^\dagger m^\dagger \rangle & -i\langle am \rangle + i\langle a^\dagger m^\dagger \rangle \\ -i\langle a^2 \rangle - i\langle a^{\dagger 2} \rangle & -\langle a^2 \rangle - \langle a^{\dagger 2} \rangle + 2\langle aa^\dagger \rangle & -i\langle am \rangle + i\langle a^\dagger m^\dagger \rangle & -\langle am \rangle - \langle a^\dagger m^\dagger \rangle \\ \langle am \rangle + \langle a^\dagger m^\dagger \rangle & -i\langle am \rangle + i\langle a^\dagger m^\dagger \rangle & \langle m^2 \rangle + \langle m^{\dagger 2} \rangle + 2\langle mm^\dagger \rangle & -i\langle m^2 \rangle - i\langle m^{\dagger 2} \rangle \\ -i\langle am \rangle + i\langle a^\dagger m^\dagger \rangle & -\langle am \rangle - \langle a^\dagger m^\dagger \rangle & -i\langle m^2 \rangle - i\langle m^{\dagger 2} \rangle & -\langle m^2 \rangle - \langle m^{\dagger 2} \rangle + 2\langle mm^\dagger \rangle \end{pmatrix} - \mathbb{I}_4. \quad (\text{S78})$$

Consequently, the second-order cumulants of the Q-function whose tomography is directly obtained by heterodyne measurement gives only access to the first term  $\mathcal{V}_Q$ , which is the normally ordered covariance matrix. One needs to subtract to it the covariance matrix of the vacuum in order to get the actual  $\mathcal{V}$ .

$$\boxed{\mathcal{V}_Q = \mathcal{V} + \mathbb{I}_4} \quad (\text{S79})$$

### ON-OFF measurement

#### Determination of amplifying setup gain $G_{amp}$

In order to access the covariance matrix of the modes  $a$  and  $m$ , we must subtract the uncorrelated noise from the amplifying setup  $h_{in}$  and determine the gain of the amplifying setup  $G_{amp}$ .

One can show the following relations assuming that the modes  $a_{in}$  and  $m_{in,1}$  are in the vacuum state at rest. First when the entanglement pulse is ON:

$$\langle A_{out}^{on} A_{out}^{on\dagger} \rangle = G_{amp} \langle a_{out,1} a_{out,1}^\dagger \rangle_{|Sq\rangle} + (G_{amp} - 1) \langle h_{in,1}^\dagger h_{in,1} \rangle_{thermal} \quad (\text{S80})$$

$$= G_{amp} (\cosh^2(r) \langle a_{in} a_{in}^\dagger \rangle_{|0\rangle} + \sinh^2(r) \langle m_{in,1}^\dagger m_{in,1} \rangle_{|0\rangle}) + (G_{amp} - 1) \langle h_{in,1}^\dagger h_{in,1} \rangle_{thermal} \quad (\text{S81})$$

$$= G_{amp} \cosh^2(r) + (G_{amp} - 1) \langle h_{in,1}^\dagger h_{in,1} \rangle_{thermal} \quad (\text{S82})$$

Then when the entanglement pulse is turned OFF:

$$\langle A_{out}^{off} A_{out}^{off\dagger} \rangle = G_{amp} \langle a_{in} a_{in}^\dagger \rangle_{|0\rangle} + (G_{amp} - 1) \langle h_{in,1}^\dagger h_{in,1} \rangle_{thermal} \quad (\text{S83})$$

$$= G_{amp} + (G_{amp} - 1) \langle h_{in,1}^\dagger h_{in,1} \rangle_{thermal}. \quad (\text{S84})$$

Consequently, we have:

$$\langle A_{out}^{on} A_{out}^{on\dagger} \rangle - \langle A_{out}^{off} A_{out}^{off\dagger} \rangle = G_{amp} (\cosh^2(r) - 1) \quad (\text{S85})$$

Here, the amplitude gain of the entanglement process  $\cosh r$  is measured independently (Fig. S9), so we can extract the gain of the amplifying setup  $G_{amp}$ :

$$G_{amp} = \frac{\langle A_{out}^{on} A_{out}^{on\dagger} \rangle - \langle A_{out}^{off} A_{out}^{off\dagger} \rangle}{\cosh^2(r) - 1} \quad (\text{S86})$$

$$\boxed{G_{amp} = \frac{1}{\cosh^2(r) - 1} \int d^2\alpha |\alpha|^2 (Q^{on}(\alpha) - Q^{off}(\alpha))} \quad (\text{S87})$$

*Reconstruction of the covariance matrix*

The measured histograms give an access to the measured normally ordered covariance matrix  $\mathcal{V}_Q^{Meas,on}$  and  $\mathcal{V}_Q^{Meas,off}$ . Without loss of generality, we suppose that the noise added by the amplifying setup is thermal i.e. uncorrelated, it corresponds to a diagonal covariance matrix.

$$\mathcal{V}_Q^{Meas,on} = \begin{pmatrix} \langle A^2 \rangle + \langle A^{\dagger 2} \rangle + 2\langle AA^\dagger \rangle & -i\langle A^2 \rangle - i\langle A^{\dagger 2} \rangle & \langle AM \rangle + \langle A^\dagger M^\dagger \rangle & -i\langle AM \rangle + i\langle A^\dagger M^\dagger \rangle \\ -i\langle A^2 \rangle - i\langle A^{\dagger 2} \rangle & -\langle A^2 \rangle - \langle A^{\dagger 2} \rangle + 2\langle AA^\dagger \rangle & -i\langle AM \rangle + i\langle A^\dagger M^\dagger \rangle & -\langle AM \rangle - \langle A^\dagger M^\dagger \rangle \\ \langle AM \rangle + \langle A^\dagger M^\dagger \rangle & -i\langle AM \rangle + i\langle A^\dagger M^\dagger \rangle & \langle M^2 \rangle + \langle M^{\dagger 2} \rangle + 2\langle MM^\dagger \rangle & -i\langle M^2 \rangle - i\langle M^{\dagger 2} \rangle \\ -i\langle AM \rangle + i\langle A^\dagger M^\dagger \rangle & -\langle AM \rangle - \langle A^\dagger M^\dagger \rangle & -i\langle M^2 \rangle - i\langle M^{\dagger 2} \rangle & -\langle M^2 \rangle - \langle M^{\dagger 2} \rangle + 2\langle MM^\dagger \rangle \end{pmatrix}_{on} \quad (S88)$$

$$= G_{amp} \begin{pmatrix} \langle a^2 \rangle + \langle a^{\dagger 2} \rangle + 2\langle aa^\dagger \rangle & -i\langle a^2 \rangle - i\langle a^{\dagger 2} \rangle & \langle am \rangle + \langle a^\dagger m^\dagger \rangle & -i\langle am \rangle + i\langle a^\dagger m^\dagger \rangle \\ -i\langle a^2 \rangle - i\langle a^{\dagger 2} \rangle & -\langle a^2 \rangle - \langle a^{\dagger 2} \rangle + 2\langle aa^\dagger \rangle & -i\langle am \rangle + i\langle a^\dagger m^\dagger \rangle & -\langle am \rangle - \langle a^\dagger m^\dagger \rangle \\ \langle am \rangle + \langle a^\dagger m^\dagger \rangle & -i\langle am \rangle + i\langle a^\dagger m^\dagger \rangle & \langle m^2 \rangle + \langle m^{\dagger 2} \rangle + 2\langle mm^\dagger \rangle & -i\langle m^2 \rangle - i\langle m^{\dagger 2} \rangle \\ -i\langle am \rangle + i\langle a^\dagger m^\dagger \rangle & -\langle am \rangle - \langle a^\dagger m^\dagger \rangle & -i\langle m^2 \rangle - i\langle m^{\dagger 2} \rangle & -\langle m^2 \rangle - \langle m^{\dagger 2} \rangle + 2\langle mm^\dagger \rangle \end{pmatrix}_{|Sq} \quad (S89)$$

$$+ (G_{amp} - 1) \begin{pmatrix} 2\langle h_{in,1}^\dagger h_{in,1} \rangle & 0 & 0 & 0 \\ 0 & 2\langle h_{in,1}^\dagger h_{in,1} \rangle & 0 & 0 \\ 0 & 0 & 2\langle h_{in,2}^\dagger h_{in,2} \rangle & 0 \\ 0 & 0 & 0 & 2\langle h_{in,2}^\dagger h_{in,2} \rangle \end{pmatrix}_{thermal} \quad (S90)$$

$$\mathcal{V}_Q^{Meas,on} = G_{amp}(\mathcal{V} + \mathbb{I}_4) + (G_{amp} - 1)\mathcal{V}^{thermal} \quad (S91)$$

and

$$\mathcal{V}_Q^{Meas,off} = \begin{pmatrix} \langle A^2 \rangle + \langle A^{\dagger 2} \rangle + 2\langle AA^\dagger \rangle & -i\langle A^2 \rangle - i\langle A^{\dagger 2} \rangle & \langle AM \rangle + \langle A^\dagger M^\dagger \rangle & -i\langle AM \rangle + i\langle A^\dagger M^\dagger \rangle \\ -i\langle A^2 \rangle - i\langle A^{\dagger 2} \rangle & -\langle A^2 \rangle - \langle A^{\dagger 2} \rangle + 2\langle AA^\dagger \rangle & -i\langle AM \rangle + i\langle A^\dagger M^\dagger \rangle & -\langle AM \rangle - \langle A^\dagger M^\dagger \rangle \\ \langle AM \rangle + \langle A^\dagger M^\dagger \rangle & -i\langle AM \rangle + i\langle A^\dagger M^\dagger \rangle & \langle M^2 \rangle + \langle M^{\dagger 2} \rangle + 2\langle MM^\dagger \rangle & -i\langle M^2 \rangle - i\langle M^{\dagger 2} \rangle \\ -i\langle AM \rangle + i\langle A^\dagger M^\dagger \rangle & -\langle AM \rangle - \langle A^\dagger M^\dagger \rangle & -i\langle M^2 \rangle - i\langle M^{\dagger 2} \rangle & -\langle M^2 \rangle - \langle M^{\dagger 2} \rangle + 2\langle MM^\dagger \rangle \end{pmatrix}_{off} \quad (S92)$$

$$= G_{amp} \begin{pmatrix} \langle a^2 \rangle + \langle a^{\dagger 2} \rangle + 2\langle aa^\dagger \rangle & -i\langle a^2 \rangle - i\langle a^{\dagger 2} \rangle & \langle am \rangle + \langle a^\dagger m^\dagger \rangle & -i\langle am \rangle + i\langle a^\dagger m^\dagger \rangle \\ -i\langle a^2 \rangle - i\langle a^{\dagger 2} \rangle & -\langle a^2 \rangle - \langle a^{\dagger 2} \rangle + 2\langle aa^\dagger \rangle & -i\langle am \rangle + i\langle a^\dagger m^\dagger \rangle & -\langle am \rangle - \langle a^\dagger m^\dagger \rangle \\ \langle am \rangle + \langle a^\dagger m^\dagger \rangle & -i\langle am \rangle + i\langle a^\dagger m^\dagger \rangle & \langle m^2 \rangle + \langle m^{\dagger 2} \rangle + 2\langle mm^\dagger \rangle & -i\langle m^2 \rangle - i\langle m^{\dagger 2} \rangle \\ -i\langle am \rangle + i\langle a^\dagger m^\dagger \rangle & -\langle am \rangle - \langle a^\dagger m^\dagger \rangle & -i\langle m^2 \rangle - i\langle m^{\dagger 2} \rangle & -\langle m^2 \rangle - \langle m^{\dagger 2} \rangle + 2\langle mm^\dagger \rangle \end{pmatrix}_{|0} \quad (S93)$$

$$+ (G_{amp} - 1) \begin{pmatrix} 2\langle h_{in,1}^\dagger h_{in,1} \rangle & 0 & 0 & 0 \\ 0 & 2\langle h_{in,1}^\dagger h_{in,1} \rangle & 0 & 0 \\ 0 & 0 & 2\langle h_{in,2}^\dagger h_{in,2} \rangle & 0 \\ 0 & 0 & 0 & 2\langle h_{in,2}^\dagger h_{in,2} \rangle \end{pmatrix}_{thermal} \quad (S94)$$

$$= G_{amp} \begin{pmatrix} 2 & 0 & 0 & 0 \\ 0 & 2 & 0 & 0 \\ 0 & 0 & 2 & 0 \\ 0 & 0 & 0 & 2 \end{pmatrix} + (G_{amp} - 1) \begin{pmatrix} 2\langle h_{in,1}^\dagger h_{in,1} \rangle & 0 & 0 & 0 \\ 0 & 2\langle h_{in,1}^\dagger h_{in,1} \rangle & 0 & 0 \\ 0 & 0 & 2\langle h_{in,2}^\dagger h_{in,2} \rangle & 0 \\ 0 & 0 & 0 & 2\langle h_{in,2}^\dagger h_{in,2} \rangle \end{pmatrix}_{thermal} \quad (S95)$$

$$\mathcal{V}_Q^{Meas,off} = 2G_{amp}\mathbb{I}_4 + (G_{amp} - 1)\mathcal{V}^{thermal} \quad (S96)$$

Consequently, knowing  $G_{amp}$ , the covariance matrix of  $(a, m)$  is given by:

$$\boxed{\mathcal{V} = \frac{1}{G_{amp}}(\mathcal{V}_Q^{Meas,on} - \mathcal{V}_Q^{Meas,off}) + \mathbb{I}_4} \quad (S97)$$

### Experimental result

Here, we present the measured histograms for an entanglement pump ON or OFF and their subtraction ON-OFF. The covariance matrices extracted from these histograms with entanglement turned ON  $\mathcal{V}_Q^{Meas,ON}/G_{amp}$ , with the entanglement turned OFF  $\mathcal{V}_Q^{Meas,OFF}/G_{amp}$  and finally the reconstructed covariance matrix  $\mathcal{V}$  as described in the previous part. Note that the noise added by the amplifying setup is uncorrelated as expected. Indeed, it only affects diagonal elements and these matrix elements reach 160. This must be compared to the vacuum fluctuations which amount to covariance terms of 1. Consequently the noise added by the amplifying setup corresponds to  $N_{add} = \langle h_{in,1}^\dagger h_{in,1} \rangle = \langle h_{in,2}^\dagger h_{in,2} \rangle \approx 160 * 1/2 = 80$  photons on average.

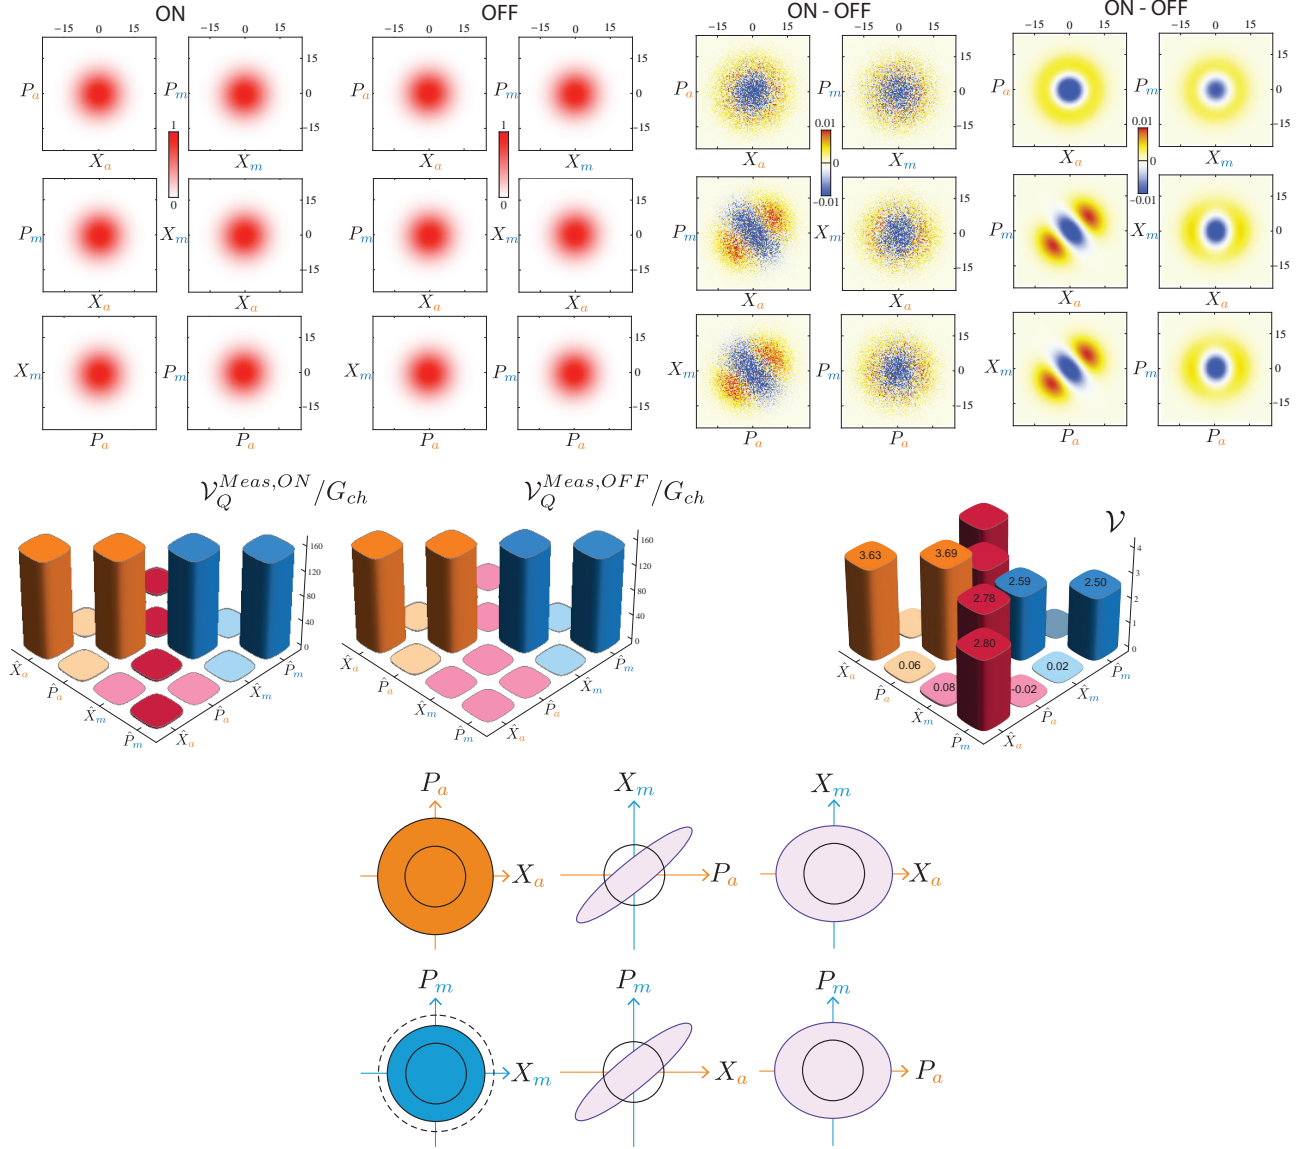

Figure S11: Histograms and corresponding covariance matrices (see text).

In order to compare the measured histograms with the ideal distribution one would get with a Gaussian state having an identical covariance matrix  $\mathcal{V}$ , we have plotted on the right side of Fig.S11 the subtraction of the corresponding Husimi-Q functions. We have also plotted the contour of the reconstructed Wigner distribution of the *EPR* state from the covariance matrix supposing that the state is Gaussian, the black circle corresponds to vacuum fluctuations.

# ENTANGLEMENT AND LOGARITHMIC NEGATIVITY

For a bipartite system, the amount of entanglement between the subsystems A and B can be quantified by means of the logarithmic negativity [7]

$$E_{\mathcal{N}}(\rho) = -\log \text{Tr}|\rho^{T_B}| \quad (\text{S98})$$

where  $\rho$  is the density matrix of the bipartite system.  $\text{Tr}|\rho^{T_B}|$  is the trace norm of the partial transpose of  $\rho$  with respect to subsystem B. If  $E_{\mathcal{N}}(\rho) > 0$  then the state is entangled, moreover it constitutes an upper bound to the distillable entanglement of the quantum state. Indeed, it corresponds to the maximal number of equivalent Bell pairs (entangled bits) that one can extract from the state by distillation.

In the case of Gaussian states, all measures of entanglement are equivalent, and they are defined by the covariance matrix. Indeed, the positivity of the partially transposed state (Peres-Horodecki PPT criterion) is necessary and sufficient for the separability of two-mode Gaussian states. Physically, it is meaningful to decompose it in four  $2 \times 2$  block matrices.

$$\mathcal{V} = \begin{pmatrix} \boldsymbol{\alpha} & \boldsymbol{\chi} \\ \boldsymbol{\chi}^T & \boldsymbol{\mu} \end{pmatrix}. \quad (\text{S99})$$

The diagonal blocks  $\boldsymbol{\alpha}$  and  $\boldsymbol{\mu}$  are the single-mode covariance matrices for  $\hat{a}$  and  $\hat{m}$  respectively. Conversely, the off-diagonal blocks  $\boldsymbol{\chi}$  correspond to the correlations between modes.

For Gaussian state, the logarithmic negativity becomes

$$E_{\mathcal{N}} = \text{Max}[-\log \nu, 0] \quad (\text{S100})$$

where

$$\nu = \sqrt{\frac{\Delta(\mathcal{V}) - \sqrt{\Delta(\mathcal{V})^2 - 4 \det \mathcal{V}}}{2}} \quad (\text{S101})$$

and

$$\Delta(\mathcal{V}) = \det \boldsymbol{\alpha} + \det \boldsymbol{\mu} - 2 \det \boldsymbol{\chi} \quad (\text{S102})$$

---

\* corresponding author: [benjamin.huard@ens.fr](mailto:benjamin.huard@ens.fr)

- [1] N. Bergeal, F. Schackert, M. Metcalfe, R. Vijay, V. E. Manucharyan, L. Frunzio, D. E. Prober, R. J. Schoelkopf, S. M. Girvin and M. H. Devoret. Phase-preserving amplification near the quantum limit with a Josephson ring modulator. *Nature* **465**, 64 (2010).
- [2] B. Abdo, A. Kamal and M. Devoret. Nondegenerate three-wave mixing with the Josephson ring modulator. *Physical Review B* **87**, 014508 (2013).
- [3] N. Bergeal, R. Vijay, V. E. Manucharyan, I. Siddiqi, R. J. Schoelkopf, S. M. Girvin and M. H. Devoret. Analog information processing at the quantum limit with a Josephson ring modulator. *Nature Physics* **6**, 296–302 (2010).
- [4] E. Flurin, N. Roch, F. Mallet, M. H. Devoret and B. Huard. Generating Entangled Microwave Radiation Over Two Transmission Lines. *Physical Review Letters* **109**, 183901 (2012).
- [5] C. M. Caves, J. Combes, Z. Jiang and S. Pandey. Quantum limits on phase-preserving linear amplifiers. *Physical Review A* **86**, 063802 (2012).
- [6] Braunstein and van Loock. Quantum information with continuous variables. *Reviews of Modern Physics* **77**, 513–577 (2005).
- [7] G. Adesso and F. Illuminati. Gaussian measures of entanglement versus negativities: Ordering of two-mode Gaussian states. *Physical Review A* **72**, 032334 (2005).
- [8] Eq. (S43) is clearly valid for low pump amplitudes  $4|\chi p_0| \ll \kappa_a$ . In fact, it remains valid for all pump amplitudes in the sense  $\pm \kappa_m$  becomes inaccurate only for pump power such that  $\gamma_{io}^m \gg \kappa_m$ .
